# Supplementary material for: Self-consistent implementation of locally scaled self-interaction-correction method
Source: arXiv:2211.03931 source file (2022-11-08)
Supplement: Supplementary file 1 [file SI.pdf]

# Supplemental information for: Self-consistent implementation of locally scaled self-interaction-correction method

Yoh Yamamoto, Tunna Baruah, Po-Hao Chang, Selim Romero, and Rajendra R. Zope

Department of Physics, University of Texas at El Paso, El Paso, Texas 79968

November 8, 2022

**Table S1** Total energies of atoms (in $E_h$) for LSIC($z$) using LSDA.

| $Z$ | LSIC($z$)-LSDA | | | | $E^{\dagger}_{Accu}$ |
|---|---|---|---|---|---|
| | Perturbative | SCF | SCF/FOD opt. | quasi-SCF | |
| 1 | -0.500 | -0.500 | -0.500 | -0.500 | -0.500 |
| 2 | -2.920 | -2.920 | -2.920 | -2.920 | -2.904 |
| 3 | -7.501 | -7.501 | -7.501 | -7.500 | -7.478 |
| 4 | -14.678 | -14.679 | -14.679 | -14.676 | -14.667 |
| 5 | -24.670 | -24.671 | -24.673 | -24.666 | -24.654 |
| 6 | -37.867 | -37.868 | -37.871 | -37.862 | -37.845 |
| 7 | -54.615 | -54.617 | -54.617 | -54.608 | -54.589 |
| 8 | -75.101 | -75.102 | -75.103 | -75.093 | -75.067 |
| 9 | -99.768 | -99.770 | -99.774 | -99.760 | -99.734 |
| 10 | -128.971 | -128.975 | -128.976 | -128.962 | -128.938 |
| 11 | -162.273 | -162.276 | -162.277 | -162.269 | -162.255 |
| 12 | -200.046 | -200.050 | -200.051 | -200.045 | -200.053 |
| 13 | -242.323 | -242.326 | -242.328 | -242.320 | -242.346 |
| 14 | -289.313 | -289.317 | -289.319 | -289.309 | -289.359 |
| 15 | -341.185 | -341.189 | -341.192 | -341.179 | -341.259 |
| 16 | -398.018 | -398.022 | -398.025 | -398.013 | -398.110 |
| 17 | -460.032 | -460.037 | -460.041 | -460.027 | -460.148 |
| 18 | -527.396 | -527.401 | -527.405 | -527.391 | -527.540 |
| MAE | 0.041 | 0.040 | 0.040 | 0.040 | |

†Reference [1]

**Table S2** Atomiaztion energies for AE6 set of data (in kcal/mol) for LSIC($z$) using LSDA..

| System | LSIC($z$)-LSDA | | | | $E^{\dagger}_{Ref}$ |
|---|---|---|---|---|---|
| | Perturbative | SCF | SCF/FOD opt. | quasi-SCF | |
| Glyoxal | 625.17 | 629.08 | 625.15 | 621.84 | 633.99 |
| Propyne | 712.48 | 713.74 | 709.34 | 701.97 | 705.06 |
| Cyclobutane | 1165.81 | 1168.54 | 1162.60 | 1146.62 | 1149.37 |
| $S_2$ | 98.82 | 99.66 | 99.30 | 99.29 | 104.25 |
| $SiH_4$ | 329.86 | 329.78 | 329.99 | 322.98 | 324.95 |
| SiO | 176.46 | 178.10 | 177.46 | 178.56 | 193.06 |
| MAE | 9.94 | 9.53 | 8.66 | 6.57 | |

†Reference [2]; reference values without spin orbit coupling effect

**Table S3** Barrier heights for BH6 set of data (in kcal/mol) for LSIC($z$) using LSDA.

| Reaction | Direction | LSIC($z$)-LSDA | | | | $E^{\dagger}_{Ref}$ |
|---|---|---|---|---|---|---|
| | | Perturbative | SCF | SCF/FOD opt. | quasi-SCF | |
| $OH + CH_4 \rightarrow CH_3 + H_2O$ | Forward | 9.3 | 7.9 | 7.9 | 6.4 | 6.7 |
| | Reverse | 19.4 | 18.0 | 17.9 | 18.9 | 19.6 |
| $H + OH \rightarrow H_2 + O$ | Forward | 10.1 | 10.1 | 10.0 | 10.3 | 10.7 |
| | Reverse | 14.3 | 12.9 | 13.0 | 14.8 | 13.1 |
| $H + H_2S \rightarrow H_2 + HS$ | Forward | 2.3 | 2.4 | 2.8 | 2.4 | 3.6 |
| | Reverse | 19.5 | 19.4 | 19.8 | 22.0 | 17.3 |
| ME | | 0.6 | 0.0 | 0.0 | 0.7 | |
| MAE | | 1.3 | 1.1 | 1.2 | 1.5 | |

$^{\dagger}$Reference [2]

**Table S4** $-\varepsilon_{HOMO}$ for a set of molecules (in eV).

| System | PBE‡ | SCAN‡ | PZSIC-LSDA‡ | LSIC($z$)-LSDA | | $IP^{\dagger}_{exp}$ |
|---|---|---|---|---|---|---|
| | | | | SCF | quasi-SCF | |
| HF | 9.63 | 10.11 | 18.47 | 14.21 | 16.13 | 16.03 |
| LiF | 6.08 | 6.36 | 13.82 | 9.91 | 11.74 | 11.3 |
| $F_2$ | 9.35 | 9.92 | 18.99 | 14.24 | 16.17 | 15.697 |
| HCl | 8.03 | 8.37 | 13.87 | 11.03 | 12.49 | 12.744 |
| LiCl | 5.83 | 6.10 | 11.08 | 8.43 | 9.73 | 9.57 |
| NaCl | 5.26 | 5.48 | 10.45 | 7.74 | 9.09 | 9.2 |
| $Cl_2$ | 7.36 | 7.69 | 13.37 | 10.32 | 11.75 | 11.481 |
| HBr | 7.45 | 7.77 | 12.62 | 10.16 | 11.42 | 11.68 |
| LiBr | 5.58 | 5.83 | 10.23 | 7.95 | 9.05 | 9.3 |
| NaBr | 5.10 | 5.30 | 9.71 | 7.39 | 8.52 | 8.3 |
| BrF | 7.46 | 7.83 | 13.25 | 10.46 | 11.84 | 11.86 |
| $Br_2$ | 6.88 | 7.21 | 12.14 | 9.53 | 10.75 | 10.517 |
| Benzene | 6.31 | 6.45 | 9.52 | 7.72 | 9.47 | 9.244 |
| Furan | 5.64 | 5.79 | 10.91 | 7.58 | 9.83 | 8.88 |
| 2-Butyne | 5.89 | 6.09 | 11.45 | 8.35 | 10.25 | 9.58 |
| $C_2H_6$ | 8.15 | 8.50 | 14.60 | 11.37 | 13.54 | 11.52 |
| $CN^-$ | -0.15 | 0.21 | 5.57 | 3.27 | 4.36 | 3.82* |
| $N_2$ | 10.29 | 10.76 | 17.80 | 14.42 | 15.80 | 15.581 |
| $H_4N_2$ | 5.71 | 6.03 | 12.32 | 9.10 | 10.96 | 8.1 |
| $H_2$ | 10.38 | 10.82 | 16.86 | 16.87 | 16.88 | 15.426 |
| $H_2O_2$ | 6.46 | 6.86 | 14.47 | 10.57 | 12.41 | 10.58 |
| BeH | 4.64 | 4.87 | 8.68 | 7.72 | 8.17 | 8.21 |
| $BH_3$ | 8.50 | 8.85 | 14.63 | 13.02 | 13.97 | 12.026 |
| Glyoxal | 6.31 | 6.65 | 13.86 | 10.03 | 11.74 | 10.2 |
| Propyne | 6.51 | 6.72 | 12.04 | 8.97 | 10.84 | 10.36 |
| Cyclobutane | 7.23 | 7.49 | 13.49 | 9.61 | 11.95 | 9.8 |
| $S_2$ | 5.81 | 6.14 | 11.31 | 8.49 | 9.67 | 9.356 |
| $SiH_4$ | 8.53 | 8.89 | 14.23 | 12.69 | 13.63 | 11 |
| SiO | 7.49 | 7.79 | 12.87 | 10.59 | 11.61 | 11.49 |
| $SO_2$ | 8.04 | 8.40 | 15.09 | 11.58 | 13.03 | 12.349 |
| $O_2$ | 6.93 | 7.55 | 15.94 | 11.43 | 13.01 | 12.07 |
| CO | 9.07 | 9.57 | 15.70 | 13.16 | 14.29 | 14.014 |
| $CO_2$ | 9.08 | 9.46 | 16.07 | 12.57 | 14.07 | 13.777 |
| $C_2H_2$ | 7.17 | 7.38 | 12.59 | 9.59 | 11.42 | 11.4 |
| $Li_2$ | 3.22 | 3.24 | 5.52 | 4.86 | 5.25 | 5.113 |
| $CH_4$ | 9.42 | 9.79 | 15.90 | 13.30 | 14.82 | 12.61 |
| $NH_3$ | 6.18 | 6.51 | 12.64 | 9.70 | 11.46 | 10.07 |
| $H_2O$ | 7.19 | 7.57 | 14.79 | 11.18 | 12.98 | 12.621 |
| MAE | 4.02 | 3.70 | 2.10 | 1.04 | 0.77 | |

‡Reference [3]

†Reference [4]

*Reference [5]

**Table S5** Bond lengths (in Å) of 12 molecules. The experiment values and deviations of theory from experiment are shown.

| Molecule | Exp† | LSDA | PZSIC-LSDA | LSIC($z$)-LSDA | | |
|---|---|---|---|---|---|---|
| | | | | Perturbative | SCF | SCF/FOD opt. |
| LiH | 1.595 | 0.007 | -0.041 | 0.004 | 0.005 | 0.004 |
| BeH | 1.343 | 0.017 | -0.032 | -0.006 | -0.006 | -0.006 |
| BH | 1.233 | 0.023 | -0.028 | -0.009 | -0.010 | -0.006 |
| $CH_4$ | 1.087 | 0.010 | -0.047 | -0.004 | -0.006 | -0.006 |
| CO | 1.128 | 0.000 | -0.040 | -0.007 | -0.007 | -0.007 |
| NH | 1.036 | 0.019 | -0.026 | -0.007 | -0.006 | -0.006 |
| NO | 1.151 | -0.003 | -0.052 | -0.009 | -0.010 | -0.009 |
| $N_2$ | 1.098 | -0.002 | -0.040 | -0.010 | -0.010 | -0.010 |
| OH | 0.970 | 0.016 | -0.023 | -0.007 | -0.007 | -0.004 |
| $O_2$ | 1.207 | 0.000 | -0.063 | -0.009 | -0.010 | -0.010 |
| HF | 0.917 | 0.016 | -0.020 | -0.004 | -0.004 | -0.002 |
| $F_2$ | 1.412 | -0.022 | -0.112 | -0.024 | -0.023 | -0.026 |
| MAE | | 0.011 | 0.044 | 0.008 | 0.009 | 0.008 |

†Reference [6]

## References


1 S. J. Chakravorty, S. R. Gwaltney, E. R. Davidson, F. A. Parpia and C. F. p Fischer, *Phys. Rev. A*, 1993, **47**, 3649–3670.

2 B. J. Lynch and D. G. Truhlar, *J. Phys. Chem. A*, 2003, **107**, 8996–8999.

3 Y. Yamamoto, C. M. Diaz, L. Basurto, K. A. Jackson, T. Baruah and R. R. Zope, *J. Chem. Phys.*, 2019, **151**, 154105.

4 P. Linstrom and W. Mallard, Eds., NIST Chemistry WebBook, NIST Standard Reference Database Number 69, National Institute of Standards and Technology, Gaithersburg MD, 20899, https://doi.org/10.18434/T4D303, (retrieved March 19, 2019).

5 K. P. Huber and G. Herzberg, *Molecular Spectra and Molecular Structure*, Van Nostrand Reinhold, New York, 1979, vol. 4. Constants of diatomic molecules.

6 D. R. Lide, *CRC handbook of chemistry and physics*, CRC press, 2004, vol. 85.
